# Supplementary material for: An Impulse-formed Navier-Stokes Solver based on Long-range Particle Flow Maps
Source: arXiv:2602.00499 source file (2026-01-31)
Supplement: Supplementary file 1 [file appendix.tex]

\section{Appendix}
\subsection{Flow Map Jacobian Advection}
\label{sec:jacobian_proof}
\subsection{Perfect Flow Map}
\label{sec:perfect_flow_map}
